# Supplementary material for: Effective Electromagnetic Wave Properties of Disordered Stealthy Hyperuniform Layered Media Beyond the Quasistatic Regime
Source: arXiv:2305.13280 ancillary file (2023-07-31)
Supplement: Supplementary file 1 [file Supplement1.pdf]

# Effective Electromagnetic Wave Properties in Disordered Stealthy Hyperuniform Layered Media Beyond the Quasistatic Regime: Supplemental Document

## 1. BACKGROUND THEORY

### A. $n$-Point Correlation Functions

A two-phase random medium is a domain of space partitioned into two disjoint regions: a phase 1 region $\mathcal{V}_1$ of volume fraction $\phi_1$ and a phase 2 region $\mathcal{V}_2$ of volume fraction $\phi_2$ [1]. The phase indicator function $\mathcal{I}^{(i)}(\mathbf{x})$ of phase $i$ for a given realization is defined as

$$\mathcal{I}^{(i)}(\mathbf{x}) = \begin{cases} 1, & \mathbf{x} \in \mathcal{V}_i, \\ 0, & \mathbf{x} \notin \mathcal{V}_i. \end{cases} \tag{S1}$$

The $n$-point correlation function $S_n^{(i)}$ for phase $i$ is defined by [1, 2]:

$$S_n^{(i)}(\mathbf{x}_1, \ldots, \mathbf{x}_n) = \left\langle \prod_{j=1}^{n} \mathcal{I}^{(i)}(\mathbf{x}_j) \right\rangle, \tag{S2}$$

where angular brackets denote an ensemble average over realizations.

For statistically homogeneous media, the $n$-point correlation functions are translationally invariant. In particular, $S_1^{(i)}(\mathbf{x}_1) = \phi_i$ and $S_2^{(i)}(\mathbf{x}_1, \mathbf{x}_2) = S_2^{(i)}(\mathbf{r})$, where $\mathbf{r} \equiv \mathbf{x}_2 - \mathbf{x}_1$. The function $S_2^{(i)}(\mathbf{r})$ for phase $i$ is simply related to the *autocovariance* function $\chi_V(\mathbf{r}) \equiv S_2^{(i)}(\mathbf{r}) - {\phi_i}^2$, which is independent of phase $i$. Thus, $\chi_V(\mathbf{r} = 0) = \phi_1\phi_2$ and, assuming the medium possesses no long-range order, $\lim_{|\mathbf{r}|\to\infty} \chi_V(\mathbf{r}) = 0$. The nonnegative spectral density $\tilde{\chi}_V(\mathbf{k})$ is the Fourier transform of $\chi_V(\mathbf{r})$ at a wavevector $\mathbf{k}$ and is proportional to scattering intensity [3] when $\mathbf{k}$ is the momentum-transfer wavevector.

### B. General Nonlocal Strong-Contrast Expansion Formalism in Three Dimensions

Here, we provide a detailed review of the nonlocal strong-contrast expansions of the effective dielectric constant tensor $\boldsymbol{\varepsilon}_e(\mathbf{k}_q, \omega)$ for statistically anisotropic two-phase composites in three dimensions derived in Ref. [4]. We consider a macroscopically large two-phase composite specimen in three dimensions embedded inside an infinitely large reference phase $q$ with the dielectric constant tensor $\boldsymbol{\varepsilon}_q$. The microstructure is perfectly general, and its characteristic inhomogeneity length scale $\xi$ is much smaller than the specimen size $L$, i.e., $\xi \ll L$. It is assumed that the applied or incident electric field $\mathbf{E}_0(\mathbf{x})$ is a plane electric wave of an angular frequency $\omega$ and a wavevector $\mathbf{k}_q$ in the reference phase $q$. While one can take $\boldsymbol{\varepsilon}_q$ to be any isotropic or anisotropic tensor that meets physical constraints, for the brevity of notation, we henceforth take the reference phase $q$ as the matrix phase (i.e., $q = 1$ or 2) of the composite unless otherwise stated. We discuss the optimal reference phase later in Sec. 2. For simplicity, we make three assumptions on phase properties: (a) both phases have real-valued and frequency-independent dielectric constants, (b) both phases are dielectrically isotropic, and (c) both phases are nonmagnetic. Due to these assumptions, the incident wavenumber $k_q$ and frequency $\omega$ are directly related by the linear dispersion relation, i.e., $k_q(\omega) \equiv |\mathbf{k}_q(\omega)| = \sqrt{\varepsilon_q}\omega/c$, where $c$ is the speed of light in vacuum. Thus, we henceforth do not explicitly indicate the $\omega$ dependence, i.e., $\boldsymbol{\varepsilon}_e(\mathbf{k}_q, \omega) = \boldsymbol{\varepsilon}_e(\mathbf{k}_q)$

In the presence of an incident wave, the resulting local electric field $\mathbf{E}(\mathbf{x})$ solves the time-harmonic vector wave equation [5]:

$$\boldsymbol{\nabla} \times \boldsymbol{\nabla} \times \mathbf{E}(\mathbf{x}) - {k_q}^2\, \mathbf{E}(\mathbf{x}) = \left(\frac{\omega}{c}\right)^2 \mathbf{P}(\mathbf{x}), \tag{S3}$$

where $\mathbf{P}(\mathbf{x})$ is the *polarization field* given by

$$\mathbf{P}(\mathbf{x}) \equiv \left[\varepsilon(\mathbf{x}) - \varepsilon_q\right] \mathbf{E}(\mathbf{x}) \tag{S4}$$

and

$$\varepsilon(\mathbf{x}) = (\varepsilon_p - \varepsilon_q)\mathcal{I}^{(p)}(\mathbf{x}) + \varepsilon_q \tag{S5}$$

is the local dielectric constant, and $\mathcal{I}^{(p)}(\mathbf{x})$ is the indicator function for phase $p$ [cf. (S1)]. The vector $\mathbf{P}(\mathbf{x})$ is the induced flux field relative to reference phase $q$ due to the presence of phase $p$ and hence is zero in the reference phase $q$ and nonzero in the 'polarized' phase $p$ ($p \neq q$).

Using the Green's function formalism, the local electric field can be expressed in terms of the following integral equation [1, 5]:

$$\mathbf{E}(\mathbf{x}) = \mathbf{E}_0(\mathbf{x}) + \int \boldsymbol{G}^{(q)}\left(\mathbf{x} - \mathbf{x}'\right) \cdot \mathbf{P}\left(\mathbf{x}'\right) \mathrm{d}\mathbf{x}', \tag{S6}$$

where $\boldsymbol{G}^{(q)}(\mathbf{r})$ is the second-rank tensor Green's function associated with the reference phase $q$ [1]; see the left-hand side of Eq. (S3). Since $\boldsymbol{G}^{(q)}\left(\mathbf{x} - \mathbf{x}'\right)$ has a singularity at $\mathbf{x} = \mathbf{x}'$, it is convenient to separate $\boldsymbol{G}^{(q)}\left(\mathbf{x} - \mathbf{x}'\right)$ into two terms:

$$\boldsymbol{G}^{(q)}(\mathbf{r}) = -\boldsymbol{D}^{(q)}\, \delta(\mathbf{r}) + \boldsymbol{H}^{(q)}(\mathbf{r}), \tag{S7}$$

where a constant second-rank tensor $\boldsymbol{D}^{(q)}$, called the source dyadic, arises from an infinitesimal region around the position of the singularity $\mathbf{x}' = \mathbf{x}$ in the Green's function, and $\boldsymbol{H}^{(q)}(\mathbf{r})$ represents the contribution outside of the "exclusion" region. In three dimensions, the principal part of the Green's function (outside the exclusion region) is

$$\boldsymbol{H}^{(q)}(\mathbf{r}) = \frac{\exp\left(ik_q r\right)}{\varepsilon_q 4\pi r^3}\left[-1 + ik_q r + (k_q r)^2\right] + \frac{\exp\left(ik_q r\right)}{\varepsilon_q 4\pi r^3}\left[3 - 3ik_q r - (k_q r)^2\right]\hat{\mathbf{r}}\hat{\mathbf{r}}, \tag{S8}$$

where $\hat{\mathbf{r}} \equiv \mathbf{r}/|\mathbf{r}|$ is a unit vector directed to $\mathbf{r}$. Since $\mathbf{E}(\mathbf{x})$ given in Eq. (S6) is independent of the choice of the exclusion region, the term $\boldsymbol{D}^{(q)}$ has to depend on the exclusion region instead [4, 6].

The nonlocal strong-contrast expansion is a series expansion of the linear fractional form of the effective dynamic dielectric constant $\boldsymbol{\varepsilon}_e\left(\mathbf{k}_q\right)$ that can be written as

$$\phi_p \boldsymbol{L}_p^{(q)} \cdot \left[\boldsymbol{L}_e\left(\mathbf{k}_q\right)\right]^{-1} \cdot \phi_p \boldsymbol{L}_p^{(q)} = \phi_p \boldsymbol{L}_p^{(q)} - \sum_{n=2}^{\infty} \boldsymbol{\mathcal{A}}_n^{(p)}\left(\mathbf{k}_q\right), \tag{S9}$$

where

$$\boldsymbol{L}_p^{(q)} \equiv \left(\varepsilon_p - \varepsilon_q\right)\left[\boldsymbol{I} + \boldsymbol{D}^{(q)}\left(\varepsilon_p - \varepsilon_q\right)\right]^{-1}, \tag{S10}$$

$$\boldsymbol{L}_e^{(q)}\left(\mathbf{k}_q\right) \equiv \left[\boldsymbol{\varepsilon}_e\left(\mathbf{k}_q\right) - \varepsilon_q \boldsymbol{I}\right] \cdot \left\{\boldsymbol{I} + \boldsymbol{D}^{(q)} \cdot \left[\boldsymbol{\varepsilon}_e\left(\mathbf{k}_q\right) - \varepsilon_q \boldsymbol{I}\right]\right\}^{-1}, \tag{S11}$$

and $\boldsymbol{\mathcal{A}}_n^{(p)}\left(\mathbf{k}_q\right)$ is a wavevector-dependent second-rank tensor that is a functional involving the set of correlation functions $S_1^{(p)}, S_2^{(p)}, \ldots, S_n^{(p)}$ and products of the principal part of the dyadic Green's function $\boldsymbol{H}^{(q)}(\mathbf{r})$. Specifically,

$$\boldsymbol{\mathcal{A}}_2^{(p)}\left(\mathbf{k}_q\right) \equiv \boldsymbol{L}_p^{(q)} \cdot \left[\int_\epsilon \mathrm{d}\mathbf{x}_1\, \boldsymbol{H}^{(q)}(\mathbf{x}_1 - \mathbf{x}_2)\, e^{-i\mathbf{k}_q \cdot (\mathbf{x}_1 - \mathbf{x}_2)}\, \chi_V(\mathbf{x}_1 - \mathbf{x}_2)\right] \cdot \boldsymbol{L}_p^{(q)}, \tag{S12}$$

$$\boldsymbol{\mathcal{A}}_n^{(p)}\left(\mathbf{k}_q\right) \equiv \left(\frac{-1}{\phi_p}\right)^{n-2} \int_\epsilon \mathrm{d}\mathbf{x}_1 \cdots \mathrm{d}\mathbf{x}_{n-1} \prod_{j=1}^{n-1}\left[\boldsymbol{L}_p^{(q)} \cdot \boldsymbol{H}^{(q)}\left(\mathbf{x}_j - \mathbf{x}_{j+1}\right) e^{-i\mathbf{k}_q \cdot (\mathbf{x}_j - \mathbf{x}_{j+1})}\right] \cdot \boldsymbol{L}_p^{(q)}\, \Delta_n^{(p)}(\mathbf{x}_1, \cdots, \mathbf{x}_n), \quad (n > 2), \tag{S13}$$

where $\int_\epsilon \mathrm{d}\mathbf{r}$ stands for the Cauchy principal value of the integral by omitting the exclusion region around the origin, and $\Delta_n^{(p)}$ is a position-dependent determinant involving $m$-point correlation

[1] The Green's function in this work (S7) differs from the one given in Ref. [5] by a multiplicative factor $(\omega/c)^2$. Thus, Eq. (S7) converges to its static counterpart in the static limit (i.e., $\omega \to 0$).

function $S_m^{(p)}$ of the polarized phase $p$ up to the $n$-point level:

$$\Delta_n^{(p)}(\mathbf{x}_1,\cdots,\mathbf{x}_n) = \begin{vmatrix} S_2^{(p)}(\mathbf{x}_1,\mathbf{x}_2) & S_1^{(p)}(\mathbf{x}_1) & \cdots & 0 \\ S_3^{(p)}(\mathbf{x}_1,\mathbf{x}_2,\mathbf{x}_3) & S_2^{(p)}(\mathbf{x}_2,\mathbf{x}_3) & \cdots & 0 \\ \vdots & \vdots & \ddots & \vdots \\ S_n^{(p)}(\mathbf{x}_1,\cdots,\mathbf{x}_n) & S_{n-1}^{(p)}(\mathbf{x}_2,\cdots,\mathbf{x}_n) & \cdots & S_2^{(p)}(\mathbf{x}_{n-1},\mathbf{x}_n) \end{vmatrix}. \tag{S14}$$

For a spherical exclusion region, $\boldsymbol{\mathcal{A}}_n^{(p)}(\mathbf{k}_q)$ is related to the coefficient $A_n^{(p)}(\mathbf{k}_q)$ in Ref. [4] as follows: $\boldsymbol{\mathcal{A}}_n^{(p)}(\mathbf{k}_q) = 3\varepsilon_q\beta_{pq}(3)^n\, A_n^{(p)}(\mathbf{k}_q)$ for $n \geq 2$, where $\beta_{pq}(3) \equiv (\varepsilon_p - \varepsilon_q)/(\varepsilon_p + 2\varepsilon_q)$ is the dielectric polarizability in three dimension. In practice, it is challenging to compute the higher-order terms $\boldsymbol{\mathcal{A}}_n^{(p)}(\mathbf{k}_q)$ for $n > 2$, and thus we focus on the truncations at the two-point level.

The strong-contrast expansion (S9) has four important features:

1. This expansion is established based on a spatially nonlocal constitutive relation, i.e., the average polarization field at position $\mathbf{x}$ depends on the average electric field at other positions around $\mathbf{x}$ [7, 8]. from the long- to intermediate-wavelength regimes, i.e., $0 \leq |\mathbf{k}_q|\xi \lesssim 1$, where $\xi$ is a characteristic inhomogeneity length scale. Specifically, the exact strong-contrast expansion (S9) relies on the following *nonlocal* constitutive relation:

$$\langle \mathbf{P}\rangle(\mathbf{x}) = \int \mathrm{d}\mathbf{x}'\, \boldsymbol{L}_e^{(q)}(\mathbf{x}-\mathbf{x}')\cdot\langle\mathbf{F}\rangle(\mathbf{x}'), \tag{S15}$$

   which is reduced to a linear product by taking the Fourier transform as follows:

$$\widetilde{\langle \mathbf{P}\rangle}(\mathbf{k}_q) = \boldsymbol{L}_e^{(q)}(\mathbf{k}_q)\cdot\widetilde{\langle\mathbf{F}\rangle}(\mathbf{k}_q). \tag{S16}$$

   This relation is equivalent to the popular nonlocal constitutive relation [4]:

$$\widetilde{\langle \mathbf{D}\rangle}(\mathbf{k}) = \varepsilon_0\,\boldsymbol{\varepsilon}_e(\mathbf{k})\cdot\widetilde{\langle\mathbf{E}\rangle}(\mathbf{k}), \tag{S17}$$

   where $\varepsilon_0$ is the dielectric permittivity of vacuum.

2. The representation (S9) exactly treats multiple scattering to all orders at a given incident wavevector $\mathbf{k}_q$ when the nonlocal homogenization theory is valid because the terms $\boldsymbol{\mathcal{A}}_n^{(p)}(\mathbf{k}_q)$ for $n = 2,\ldots$ in this series explicitly account for complete microstructural information (the infinite set of $S_2, S_3, \ldots$) to infinite order.

3. A choice for the shape of the infinitesimal exclusion region determines symmetries of a tensor $\boldsymbol{D}^{(q)}$. We present some important examples below: [4, 6]

$$\boldsymbol{D}^{(q)} = \begin{cases} \frac{1}{3\varepsilon_q}\boldsymbol{I}, & \text{spherical exclusion volume} \\ \frac{1}{\varepsilon_q}\hat{\mathbf{z}}\hat{\mathbf{z}}, & \text{disk-like exclusion volume perpendicular to the } z \text{ axis} \\ \frac{1}{2\varepsilon_q}(\boldsymbol{I}-\hat{\mathbf{z}}\hat{\mathbf{z}}), & \text{needle-like exclusion volume aligned with the } z \text{ axis} \end{cases}, \tag{S18}$$

   where its trace $\mathrm{Tr}\left[\boldsymbol{D}^{(q)}\right]$ is always independent of the exclusion volume shape [6]: $\mathrm{Tr}\left[\boldsymbol{D}^{(q)}\right] \equiv \boldsymbol{I}:\boldsymbol{D}^{(q)} = 1/\varepsilon_q$. Thus, a different choice of the exclusion-region shape leads to a different expansion parameter $\boldsymbol{L}_p^{(q)}$ and expansion with significantly different convergence properties. For this reason, different from the standard multiple-scattering theory [9–13], one can naturally 'tune' the general series expansions to obtain distinctly different approximations suited for certain classes of microstructures.

4. The left-handed side of this series is a linear fractional transformation of $\boldsymbol{\varepsilon}_e(\mathbf{k}_q)$ rather than $\boldsymbol{\varepsilon}_e(\mathbf{k}_q)$ itself, which leads to the rapid convergence of the strong-contrast expansions in that the lower-order truncations of the series can well approximate higher-order functionals (i.e., higher-order diagrams) of the exact series to all orders in terms of lower-order diagrams; see Sec. IIIB of Ref. [4] for details.

It is useful to consider the Fourier representation of the coefficient $\boldsymbol{\mathcal{A}}_n^{(p)}(\mathbf{k}_q)$ given in Eq. (S12) and Eq. (S13) because the Fourier transform of the dyadic Green's function given in Eq. (S7) is particularly simple and concise:

$$\tilde{G}_{ij}^{(q)}(\mathbf{k}) = \frac{1}{\varepsilon_q}\frac{{k_q}^2\delta_{ij} - k_i k_j}{k^2 - {k_q}^2}. \tag{S19}$$

Note that Eq. (S19) is independent of the shape of the exclusion region, which stands in contrast to the shape-dependent Fourier transform of $H_{ij}^{(q)}(\mathbf{r})$:

$$\tilde{\boldsymbol{H}}^{(q)}(\mathbf{k}) = \tilde{\boldsymbol{G}}^{(q)}(\mathbf{k}) + \boldsymbol{D}^{(q)} = \frac{1}{\varepsilon_q}\frac{{k_q}^2\boldsymbol{I} - \mathbf{k}\mathbf{k}}{k^2 - {k_q}^2} + \boldsymbol{D}^{(q)}. \tag{S20}$$

Here, we present the Fourier representations of the first two coefficients $\boldsymbol{\mathcal{A}}_2^{(p)}(\mathbf{k}_q)$ and $\boldsymbol{\mathcal{A}}_3^{(p)}(\mathbf{k}_q)$:

$$\begin{aligned}
\boldsymbol{\mathcal{A}}_2^{(p)}(\mathbf{k}_q) \equiv& \boldsymbol{L}_p^{(q)} \cdot \left\{\frac{1}{(2\pi)^3}\int \mathrm{d}\mathbf{q} \left[\tilde{\boldsymbol{G}}^{(q)}(\mathbf{k}_q + \mathbf{q}) + \boldsymbol{D}^{(q)}\right]\tilde{\chi}_V(\mathbf{q})\right\} \cdot \boldsymbol{L}_p^{(q)} \\
=& \boldsymbol{L}_p^{(q)} \cdot \left\{\frac{1}{(2\pi)^3}\int \mathrm{d}\mathbf{q} \left[\frac{1}{\varepsilon_q}\frac{{k_q}^2\boldsymbol{I} - (\mathbf{q}+\mathbf{k}_q)(\mathbf{q}+\mathbf{k}_q)}{\left|\mathbf{q}+\mathbf{k}_q\right|^2 - {k_q}^2} + \boldsymbol{D}^{(q)}\right]\tilde{\chi}_V(\mathbf{q})\right\} \cdot \boldsymbol{L}_p^{(q)},
\end{aligned} \tag{S21}$$

$$\begin{aligned}
\boldsymbol{\mathcal{A}}_3^{(p)}(\mathbf{k}_q) =& \frac{-1}{\phi_p}\int_\epsilon \mathrm{d}\mathbf{x}_1\,\mathrm{d}\mathbf{x}_2 \left[\boldsymbol{L}_p^{(q)} \cdot \boldsymbol{H}^{(q)}(\mathbf{x}_1 - \mathbf{x}_2)\, e^{-i\mathbf{k}_q\cdot(\mathbf{x}_1-\mathbf{x}_2)} \cdot \boldsymbol{L}_p^{(q)} \cdot \boldsymbol{H}^{(q)}(\mathbf{x}_2 - \mathbf{x}_3)\, e^{-i\mathbf{k}_q\cdot(\mathbf{x}_2-\mathbf{x}_3)}\right] \\
&\cdot \boldsymbol{L}_p^{(q)}\,\Delta_3^{(p)}(\mathbf{x}_1, \mathbf{x}_2, \mathbf{x}_3), \\
=& \frac{-1}{\phi_p}\frac{1}{(2\pi)^6}\int \mathrm{d}\mathbf{q}_1\,\mathrm{d}\mathbf{q}_2 \left[\boldsymbol{L}_p^{(q)} \cdot \tilde{\boldsymbol{H}}^{(q)}(\mathbf{k}_q + \mathbf{q}_1) \cdot \boldsymbol{L}_p^{(q)} \cdot \tilde{\boldsymbol{H}}^{(q)}(\mathbf{k}_q + \mathbf{q}_2)\right] \cdot \boldsymbol{L}_p^{(q)}\,\tilde{\Delta}_3^{(p)}(-\mathbf{q}_1, -\mathbf{q}_2),
\end{aligned} \tag{S22}$$

where we have used the convolution theorem, and

$$\tilde{\Delta}_3^{(p)}(\mathbf{q}_1, \mathbf{q}_2) \equiv \int \mathrm{d}\mathbf{r}\,\mathrm{d}\mathbf{s}\, e^{-i\mathbf{q}_1\cdot\mathbf{r}} e^{-i\mathbf{q}_2\cdot\mathbf{s}}\left[S_2^{(p)}(\mathbf{r})\, S_2^{(p)}(\mathbf{s}) - \phi_p\, S_3^{(p)}(\mathbf{r}, \mathbf{t})\right] \tag{S23}$$

$$\begin{aligned}
=& -\phi_p \left\langle \delta\tilde{\mathcal{I}}^{(p)}(-\mathbf{q}_1)\, \delta\tilde{\mathcal{I}}^{(p)}(\mathbf{q}_1 - \mathbf{q}_2)\, \delta\tilde{\mathcal{I}}^{(p)}(\mathbf{q}_2)\right\rangle \\
&- {\phi_p}^2 (2\pi)^3\, \delta(\mathbf{q}_1 - \mathbf{q}_2)\, \tilde{\chi}_V(\mathbf{q}_2) + \tilde{\chi}_V(\mathbf{q}_1)\, \tilde{\chi}_V(\mathbf{q}_2),
\end{aligned} \tag{S24}$$

where $\mathbf{r} \equiv \mathbf{x}_1 - \mathbf{x}_2$ and $\mathbf{t} \equiv \mathbf{x}_2 - \mathbf{x}_3$, and $\delta\tilde{I}^{(p)}(\mathbf{q})$ is the Fourier transform of $\mathcal{I}^{(p)}(\mathbf{x}) - \phi_p$, given in Eq. (S1).

### C. Strong-Fluctuation Theory

Here, we briefly compare the strong-contrast expansion formalism and the strong-property-fluctuation theory studies in Refs. [14–16]. Indeed, the strong-fluctuation theory in these three papers corresponds to a special case of our strong-contrast expansion. Both theories rely on the same treatment for the singularity of the dyadic Green's function and the same constitutive relation (whether they are local or nonlocal). However, they differ in the ways to expand the key quantity, the mass operator $\boldsymbol{\Sigma}$ or, equivalently, the effective polarizability tensor $\boldsymbol{L}_e^{(q)}$, where the superscript $q$ indicates the reference phase, which is different from phases 1 or 2 in general. The strong-fluctuation theory expands $\boldsymbol{\Sigma}$ as follows:

$$\begin{aligned}
\boldsymbol{\Sigma}(\mathbf{x} - \mathbf{x}') =& \left\langle \boldsymbol{L}^{(q)}(\mathbf{x})\right\rangle \delta(\mathbf{x} - \mathbf{x}') + \left\langle \boldsymbol{L}^{(q)}(\mathbf{x}) \cdot \boldsymbol{H}^{(q)}(\mathbf{x} - \mathbf{x}') \cdot \boldsymbol{L}^{(q)}(\mathbf{x}')\right\rangle \\
&+ \int_\epsilon \mathrm{d}\mathbf{r}_1 \left\langle \boldsymbol{L}^{(q)}(\mathbf{x}) \cdot \boldsymbol{H}^{(q)}(\mathbf{x} - \mathbf{x}_1) \cdot \boldsymbol{L}^{(q)}(\mathbf{x}_1) \cdot \boldsymbol{H}^{(q)}(\mathbf{x}_1 - \mathbf{x}') \cdot \boldsymbol{L}^{(q)}(\mathbf{x}')\right\rangle + \ldots,
\end{aligned} \tag{S25}$$

where $\langle\cdot\rangle$ is an ensemble average, $\boldsymbol{L}^{(q)}(\mathbf{x})$ is the local polarizability tensor relative to the reference phase $q$ defined as

$$\boldsymbol{L}^{(q)}(\mathbf{x}) \equiv \boldsymbol{L}_1^{(q)}\,\mathcal{I}^{(1)}(\mathbf{x}) + \boldsymbol{L}_2^{(q)}\,\mathcal{I}^{(2)}(\mathbf{x}), \tag{S26}$$

and $\mathcal{I}^{(i)}(\mathbf{x})$ is the phase indicator function of phase $i$ defined in Eq. (S1). The strong-fluctuation expansion (S25) requires renormalization because each integral is conditionally convergent. Specifically, one should choose the reference phase $q$ satisfying the following condition:

$$\left\langle \boldsymbol{L}^{(q)}(\mathbf{x}) \right\rangle = \boldsymbol{L}_1^{(q)}\phi_1 + \boldsymbol{L}_2^{(q)}\phi_2 = 0. \tag{S27}$$

Instead, the strong-contrast expansion expands the inverse of $\mathbf{\Sigma}$ as follows:

$$\begin{aligned}
[\boldsymbol{L}_e^{(q)}(\mathbf{x}-\mathbf{x}')]^{-1} =&[\mathbf{\Sigma}(\mathbf{x}-\mathbf{x}')]^{-1} + \boldsymbol{H}^{(q)}(\mathbf{x}-\mathbf{x}') \\
=&[\left\langle \boldsymbol{L}^{(q)}(\mathbf{x})\right\rangle]^{-1}\delta(\mathbf{x}-\mathbf{x}') - [\left\langle \boldsymbol{L}^{(q)}(\mathbf{x})\right\rangle]^{-1} \\
&\cdot \left[\left\langle \boldsymbol{L}^{(q)}(\mathbf{x})\cdot \boldsymbol{H}^{(q)}(\mathbf{x}-\mathbf{x}')\cdot \boldsymbol{L}^{(q)}(\mathbf{x}')\right\rangle - \left\langle \boldsymbol{L}^{(q)}(\mathbf{x})\right\rangle \cdot \boldsymbol{H}^{(q)}(\mathbf{x}-\mathbf{x}')\cdot \left\langle \boldsymbol{L}^{(q)}(\mathbf{x}')\right\rangle\right]\cdot [\left\langle \boldsymbol{L}^{(q)}(\mathbf{x}')\right\rangle]^{-1} \\
&- \ldots,
\end{aligned} \tag{S28}$$

which is written up to the second-order term. This expansion is simplified to Eq. (S9) if we take the reference phase to be the matrix phase, i.e., $q = 1, 2$. Importantly, unlike the integrals in Eq. (S25), the corresponding integrals in Eq. (S28) are absolutely convergent regardless of the choice of reference phase [1, 4].

## 2. MULTIPLE-SCATTERING APPROXIMATIONS FOR LAYERED MEDIA

Here, we explain in detail how to extract from the exact strong-contrast expansion (S9) accurate multiple-scattering approximations of $\boldsymbol{\varepsilon}_e(\mathbf{k}_q)$ for layered media by truncating the expansion at the $n$-point level. We focus here on such a formula at the two-point level that depends on the spectral density $\tilde{\chi}_V(\mathbf{k})$. We begin by describing how to utilize the symmetries of layered media. We then apply these symmetries to the general multiple-scattering approximations for layered media at the $n$-point level. We eventually derive the closed-form formulas at the two-point level.

Layered media have rotational symmetry around the $z$-axis and translational symmetry along the $x$−$y$ plane; see Fig. 1 in the main text. Due to the symmetries, the $n$-point correlation function depends solely on the $z$ coordinates of relative positions and thus can be reduced to that in one dimension: $S_n^{(i)}(\mathbf{x}_1,\ldots,\mathbf{x}_n) = S_n^{(i)}(z_2-z_1,\ldots,z_n-z_1)$. Similarly, the corresponding spectral density becomes

$$\tilde{\chi}_V(\mathbf{k}) = (2\pi)^2\,\delta(k_x)\,\delta(k_y)\,\tilde{\chi}_V(k_z)\,, \tag{S29}$$

where $\delta(k)$ is the one-dimensional Dirac delta function. For 1D packings consisting of nonoverlapping and identical rods of radius $a$ at number density $\rho$, the spectral density $\tilde{\chi}_V(k_z)$ is directly related to the structure factor $S(k_z)$ of the rod centers [1, 17]:

$$\tilde{\chi}_V(k_z) = \phi_2 \frac{2\sin^2(k_z a)}{{k_z}^2 a} S(k_z)\,, \tag{S30}$$

where $\phi_2 = 2\rho a$ is the *packing fraction* (fraction of space covered by the rods). We also use feature 4 of the strong-contrast expansion to utilize the symmetries of layered media. To do so, we choose a disk-like exclusion region normal to the $z$-axis, leading to

$$\boldsymbol{D}^{(q)} = \frac{1}{\varepsilon_q}\hat{\mathbf{z}}\hat{\mathbf{z}}. \tag{S31}$$

Substituting Eq. (S31) into Eq. (S10) yields

$$\boldsymbol{L}_p^{(q)} = \beta_{pq}\left[\varepsilon_p(\boldsymbol{I}-\hat{\mathbf{z}}\hat{\mathbf{z}}) + \varepsilon_q\hat{\mathbf{z}}\hat{\mathbf{z}}\right], \tag{S32}$$

where $\hat{\mathbf{z}}$ is a unit vector along the $z$-direction and $\beta_{pq}$ is the one-dimensional counterpart of the *dielectric polarizability*, defined as $\beta_{pq} \equiv 1 - \varepsilon_q/\varepsilon_p$.

## A. Extracting Multiple-Scattering Approximations

One can obtain multiple-scattering approximations for the general statistically anisotropic media by substituting Eq. (S31) and Eq. (S32) to the $n$th-order truncation of the exact series given in Eq. (S9), i.e.,

$$\phi_p \boldsymbol{L}_p^{(q)} \cdot [\boldsymbol{L}_e(\mathbf{k}_q)]^{-1} \cdot \phi_p \boldsymbol{L}_p^{(q)} = \phi_p \boldsymbol{L}_p^{(q)} - \boldsymbol{\mathcal{A}}_2^{(p)}(\mathbf{k}_q) - \boldsymbol{\mathcal{A}}_3^{(p)}(\mathbf{k}_q) - \ldots - \boldsymbol{\mathcal{A}}_n^{(p)}(\mathbf{k}_q) \,. \tag{S33}$$

For simplicity, we restrict ourselves to the case where the wave is incident normally into the media ($\mathbf{k}_q = k_q \hat{\mathbf{z}}$), and thus the wavenumber $k_q$ henceforth is an independent variable instead of $\mathbf{k}_q$. Furthermore, we can decompose the tensor $\boldsymbol{\varepsilon}_e(k_q)$ into two orthogonal components $\varepsilon_e^{\perp}(k_q)$ and $\varepsilon_e^{z}(k_q)$ for the transverse and longitudinal polarizations, respectively, as follows:

$$\boldsymbol{\varepsilon}_e(k_q) = \varepsilon_e^{\perp}(k_q)\,(\boldsymbol{I} - \hat{\mathbf{z}}\hat{\mathbf{z}}) + \varepsilon_e^{z}(k_q)\,\hat{\mathbf{z}}\hat{\mathbf{z}}. \tag{S34}$$

Substituting Eq. (S34) and Eq. (S32) into Eq. (S11) yields the left-handed side of Eq. (S33) for layered media

$$\phi_p \boldsymbol{L}_p^{(q)} \cdot \boldsymbol{L}_e(k_q)^{-1} \cdot \phi_p \boldsymbol{L}_p^{(q)} = \frac{(\phi_p \varepsilon_p \beta_{pq})^2}{\varepsilon_q(\varepsilon_e^{\perp}(k_q)/\varepsilon_q - 1)}(\boldsymbol{I} - \hat{\mathbf{z}}\hat{\mathbf{z}}) + \frac{(\phi_p \varepsilon_q \beta_{pq})^2}{\varepsilon_q(1 - \varepsilon_q/\varepsilon_e^{z}(k_q))}\hat{\mathbf{z}}\hat{\mathbf{z}}. \tag{S35}$$

Thus, the multiple-scattering approximations for 3D layered media are given as

$$\begin{aligned} &\frac{(\phi_p \varepsilon_p \beta_{pq})^2}{\varepsilon_q[\varepsilon_e^{\perp}(k_q)/\varepsilon_q - 1]}(\boldsymbol{I} - \hat{\mathbf{z}}\hat{\mathbf{z}}) + \frac{(\phi_p \varepsilon_q \beta_{pq})^2}{\varepsilon_q[1 - \varepsilon_q/\varepsilon_e^{z}(k_q)]}\hat{\mathbf{z}}\hat{\mathbf{z}} \\ =&\phi_p \beta_{pq}\left[\varepsilon_p(\boldsymbol{I} - \hat{\mathbf{z}}\hat{\mathbf{z}}) + \varepsilon_q \hat{\mathbf{z}}\hat{\mathbf{z}}\right] - \boldsymbol{\mathcal{A}}_2^{(p)}(k_q) - \boldsymbol{\mathcal{A}}_3^{(p)}(k_q) - \ldots - \boldsymbol{\mathcal{A}}_n^{(p)}(k_q) \,. \end{aligned} \tag{S36}$$

From now on, we focus on such a formula at the two-point level. To do so, we derive the explicit expression of $\boldsymbol{\mathcal{A}}_2^{(p)}(\mathbf{k}_q = k_q \hat{\mathbf{z}})$ for stratified media. Using Eqs. (S31) and (S32), we first rewrite Eq. (S20) as $\tilde{\boldsymbol{H}}^{(q)}(\mathbf{k}) = \frac{1}{\varepsilon_q}\left(\frac{k_q{}^2 \boldsymbol{I} - \mathbf{k}\mathbf{k}}{k^2 - k_q{}^2} + \hat{\mathbf{z}}\hat{\mathbf{z}}\right)$. After a brief algebra, we obtain

$$\begin{aligned} \boldsymbol{L}_p^{(q)} \cdot \tilde{\boldsymbol{H}}^{(q)}(\mathbf{k}) \cdot \boldsymbol{L}_p^{(q)} =& \frac{1}{\varepsilon_q}\frac{\beta_{pq}{}^2}{k^2 - k_q{}^2}\Big(\varepsilon_p{}^2\left\{k_q{}^2(\boldsymbol{I} - \hat{\mathbf{z}}\hat{\mathbf{z}}) - [\mathbf{k}]_{\perp}[\mathbf{k}]_{\perp}\right\} - \varepsilon_q \varepsilon_p k_z(\hat{\mathbf{z}}[\mathbf{k}]_{\perp} + [\mathbf{k}]_{\perp}\hat{\mathbf{z}}) \\ &+ \varepsilon_q{}^2\left(k_q{}^2 - k_z{}^2\right)\hat{\mathbf{z}}\hat{\mathbf{z}}\Big) + \varepsilon_q \beta_{pq}{}^2 \hat{\mathbf{z}}\hat{\mathbf{z}}, \end{aligned} \tag{S37}$$

where for a vector $k$, $k_z \equiv \mathbf{k} \cdot \hat{\mathbf{z}}$ and $[\mathbf{k}]_{\perp} \equiv \mathbf{k} \cdot (\boldsymbol{I} - \hat{\mathbf{z}}\hat{\mathbf{z}}) = k_x \hat{\mathbf{x}} + k_y \hat{\mathbf{y}}$. Expression for $\boldsymbol{\mathcal{A}}_2^{(p)}(k_q)$ is obtained by substituting Eq. (S29) and Eq. (S37) into Eq. (S21):

$$\begin{aligned} \boldsymbol{\mathcal{A}}_2^{(p)}(k_q) =& \frac{1}{(2\pi)^3}\int \mathrm{d}\mathbf{q}\, \boldsymbol{L}_p^{(q)} \cdot \tilde{\boldsymbol{H}}^{(q)}(k_q \hat{\mathbf{z}} + \mathbf{q}) \cdot \boldsymbol{L}_p^{(q)}\, \tilde{\chi}_V(\mathbf{q}) \\ =& \frac{1}{2\pi}\int_{-\infty}^{\infty} \mathrm{d}q_z \left[\frac{1}{\varepsilon_q}\frac{\beta_{pq}{}^2}{(q_z + k_q)^2 - k_q{}^2}\left(\varepsilon_p{}^2 k_q{}^2(\boldsymbol{I} - \hat{\mathbf{z}}\hat{\mathbf{z}}) + \varepsilon_q{}^2\left(k_q{}^2 - (q_z + k_q)^2\right)\hat{\mathbf{z}}\hat{\mathbf{z}}\right) + \varepsilon_q \beta_{pq}{}^2 \hat{\mathbf{z}}\hat{\mathbf{z}}\right] \tilde{\chi}_V(q_z) \\ =& \frac{(\varepsilon_p \beta_{pq})^2}{\varepsilon_q} F^{(1\mathrm{D})}(k_q)\,(\boldsymbol{I} - \hat{\mathbf{z}}\hat{\mathbf{z}}), \end{aligned} \tag{S38}$$

where $F^{(1\mathrm{D})}(k_q)$ is the *nonlocal attenuation function* for 1D two-phase composite defined as

$$F^{(1\mathrm{D})}(k_q) \equiv \frac{k_q{}^2}{2\pi}\int_{-\infty}^{\infty} \mathrm{d}q_z\, \frac{\tilde{\chi}_V(q_z)}{(q_z + k_q)^2 - k_q{}^2}, \tag{S39}$$

whose higher-dimensional counterparts were derived in Ref. [4]. Substituting Eq. (S38) into Eq. (S36) yields the strong-contrast approximation for layered media at the two-point level:

$$\begin{aligned} &\frac{(\phi_p \varepsilon_p \beta_{pq})^2}{\varepsilon_q[\varepsilon_e^{\perp}(k_q)/\varepsilon_q - 1]}(\boldsymbol{I} - \hat{\mathbf{z}}\hat{\mathbf{z}}) + \frac{(\phi_p \varepsilon_q \beta_{pq})^2}{\varepsilon_q[1 - \varepsilon_q/\varepsilon_e^{z}(k_q)]}\hat{\mathbf{z}}\hat{\mathbf{z}} \\ =&\phi_p \beta_{pq}\left[\varepsilon_p(\boldsymbol{I} - \hat{\mathbf{z}}\hat{\mathbf{z}}) + \varepsilon_q \hat{\mathbf{z}}\hat{\mathbf{z}}\right] - \frac{\varepsilon_p^2 \beta_{pq}{}^2}{\varepsilon_q} F^{(1\mathrm{D})}(k_q)(\boldsymbol{I} - \hat{\mathbf{z}}\hat{\mathbf{z}}), \end{aligned} \tag{S40}$$

which is decomposed into two approximate formulas:

$$\varepsilon_e^{\perp}\left(k_q\right) = \varepsilon_q\left[1+\frac{{\phi_p}^2(\varepsilon_p/\varepsilon_q)\beta_{pq}}{\phi_p-(\varepsilon_p\beta_{pq})\,F^{(1\mathrm{D})}\left(k_q\right)/\varepsilon_q}\right], \tag{S41}$$

$$\varepsilon_e^{z}\left(k_q\right) = \frac{\varepsilon_q}{1-\phi_p\beta_{pq}}. \tag{S42}$$

Note that because of the nonlocal attenuation function $F^{(1\mathrm{D})}\left(k_q\right)$, $\varepsilon_e^{\perp}\left(k_q\right)$ given in Eq. (S41) is a complex-valued quantity dependent on wavenumber $k_q$, implying that the media can be lossy due to scatterings from inhomogeneities. By contrast, $\varepsilon_e^{z}\left(k_q\right)$ is independent of $k_q$, reflecting the fact that a traveling longitudinal wave cannot exist in the case of normal incidence. We call Eq. (S41) the *non-scaled* strong-contrast approximation, which was not considered in the main text. Recall that the approximate formulas given in Eq. (S41) and Eq. (S42) are derived when the reference phase is taken to be the matrix phase $q(=1,2)$.

While the dielectric constant tensor $\boldsymbol{\varepsilon}_q$ of the reference phase $q$ does not affect the 'exact' value of the effective tensor $\boldsymbol{\varepsilon}_e\left(\mathbf{k}_q\right)$ given by the full strong-contrast expansion, $\boldsymbol{\varepsilon}_q$ does affect the convergence rate of the full expansion. Thus, the choice of the reference phase can improve or worsen the accuracy of the lower-order truncations (or approximations) of the series for $\boldsymbol{\varepsilon}_e\left(\mathbf{k}_q\right)$. The fastest convergence is achieved for the optimal reference phase (denoted by phase $I$) satisfying the condition (S27), which makes the dielectric tensor $\boldsymbol{\varepsilon}_I$ identical to the effective static dielectric constant of the layered media if $\boldsymbol{D}^{(I)} = {\boldsymbol{\varepsilon}_I}^{-1}\hat{\mathbf{z}}\hat{\mathbf{z}}$;

$$\boldsymbol{\varepsilon}_I = \langle\varepsilon\rangle\left(\boldsymbol{I}-\hat{\mathbf{z}}\hat{\mathbf{z}}\right) + \langle 1/\varepsilon\rangle^{-1}\hat{\mathbf{z}}\hat{\mathbf{z}} = \varepsilon_e^{\perp}(0)\left(\boldsymbol{I}-\hat{\mathbf{z}}\hat{\mathbf{z}}\right)+\varepsilon_e^{z}(0)\,\hat{\mathbf{z}}\hat{\mathbf{z}}, \tag{S43}$$

where $\langle\varepsilon\rangle \equiv \phi_1\varepsilon_1+\phi_2\varepsilon_2$ and $\langle 1/\varepsilon\rangle \equiv \phi_1/\varepsilon_1+\phi_2/\varepsilon_2$. Since $\boldsymbol{\varepsilon}_I$ is very close (but not identical) to the effective dynamic dielectric constant $\boldsymbol{\varepsilon}_e\left(\mathbf{k}_q\right)$ for the composite embedded in such a reference phase ($q=I$), the scattering becomes very weak through all orders so that the series converges very rapidly [14–16]. Application of such a renormalization to the strong-contrast approximation (S41) is equivalent to replacing the Green's function $\tilde{\boldsymbol{H}}^{(q)}(\mathbf{k})$ for the matrix phase $q$ in Eq. (S38) with $\tilde{\boldsymbol{H}}^{(I)}(\mathbf{k})$ for the reference phase with $\boldsymbol{\varepsilon}_I$ given by Eq. (S43) and yields the *scaled* (or renormalized) strong-contrast approximation for disordered layered media:

$$\varepsilon_e^{\perp}\left(k_q\right) = \varepsilon_q\left[1+\frac{{\phi_p}^2(\varepsilon_p/\varepsilon_q)\beta_{pq}}{\phi_p-(\varepsilon_p\beta_{pq})\,F^{(1\mathrm{D})}\left(k_q\sqrt{\langle\varepsilon\rangle/\varepsilon_q}\right)/\langle\varepsilon\rangle}\right], \tag{S44}$$

where $\langle\varepsilon\rangle \equiv \phi_1\varepsilon_1+\phi_2\varepsilon_2$. Note that the prescribed renormalization is equivalent to the effective Green's function argument used in Ref. [4] because $\tilde{\boldsymbol{H}}^{(I)}(\mathbf{k})$ is the leading-order approximation of the effective Green's function.

### B. Nonlocal Attenuation Function

The nonlocal attenuation function for 1D composites, defined in Eq. (S39), also can be written as

$$F^{(1\mathrm{D})}\left(k_q\right) = \frac{{k_q}^2}{\pi}\,\mathrm{p.v.}\int_0^{\infty}\mathrm{d}q_z\,\frac{\tilde{\chi}_V\left(q_z\right)}{{q_z}^2-(2k_q)^2}+\frac{ik_q}{4}\left[\tilde{\chi}_V(0)+\tilde{\chi}_V\left(2k_q\right)\right] \tag{S45}$$

$$= \frac{ik_q}{2}\int_0^{\infty}\mathrm{d}z\,\chi_V(z)\left(e^{2ik_q z}+1\right), \tag{S46}$$

which are the Fourier- and direct-space representations, respectively, and p.v. stands for the Cauchy principal value of an improper integral. Here, we derive Eq. (S45) and Eq. (S46) from Eq. (S39). The Fourier-space representation (S45) is obtained as follows:

$$\begin{aligned} F^{(1\mathrm{D})}(k) &= \frac{k^2}{2\pi}\int_{-\infty}^{\infty}\mathrm{d}q_z\,\frac{\tilde{\chi}_V\left(q_z\right)}{(q_z+k)^2-k^2} \\ &= \frac{k}{2\pi}\frac{1}{2}\int_{-\infty}^{\infty}\mathrm{d}q_z\left[\frac{1}{q_z}-\frac{1}{q_z-(-2k-i\epsilon)}\right]\tilde{\chi}_V\left(q_z\right) \\ &= \frac{k}{4\pi}\left[-\mathrm{p.v.}\int_{-\infty}^{\infty}\mathrm{d}q_z\,\frac{\tilde{\chi}_V\left(q_z\right)}{q_z+2k}\pm i\pi\,\tilde{\chi}_V(0)+i\pi\,\tilde{\chi}_V(-2k)\right], \end{aligned} \tag{S47}$$

where $\epsilon$ stands for an infinitesimally small positive number, and we applied the Sokhotski–Plemelj theorem, i.e.,

$$\int_{-\infty}^{\infty} \frac{f(x)}{x-x'}\,\mathrm{d}x = \lim_{\epsilon\to 0^+}\int_{-\infty}^{\infty} \frac{f(x)}{x-(x'\pm i\epsilon)}\,\mathrm{d}x = \text{p.v.}\int_{-\infty}^{\infty} \frac{f(x)}{x-x'}\,\mathrm{d}x \pm i\pi f(x')\,. \tag{S48}$$

In Eq. (S47), one should choose + sign because the imaginary part should have an identical sign at any $k$. Since the spectral density is an even function of $k$, one can rewrite Eq. (S47) as follows:

$$\begin{aligned} F^{(1\mathrm{D})}(k) &= \frac{k}{4\pi}\left\{-\text{p.v.}\int_0^{\infty}\mathrm{d}q_z\left(\frac{1}{q_z+2k}+\frac{1}{-q_z+2k}\right)\tilde{\chi}_V(q_z) + i\pi[\tilde{\chi}_V(0)+\tilde{\chi}_V(-2k)]\right\} \\ &= \frac{k^2}{\pi}\text{p.v.}\int_0^{\infty}\mathrm{d}q_z\,\frac{\tilde{\chi}_V(q_z)}{{q_z}^2-(2k)^2} + \frac{ik}{4}[\tilde{\chi}_V(0)+\tilde{\chi}_V(2k)]. \end{aligned} \tag{S49}$$

The direct-space representation (S46) is obtained by applying the Plancherel theorem to Eq. (S39):

$$\begin{aligned} F^{(1\mathrm{D})}(k) =& k^2\int_{-\infty}^{\infty}\mathrm{d}z\,\chi_V(z)\,\text{F.T.}^{-1}\left[\frac{1}{|q+k|^2-k^2}\right](z) \\ =& k^2\int_{-\infty}^{\infty}\mathrm{d}z\,\chi_V(z)\,e^{-ikz}\,\text{F.T.}^{-1}\left[\frac{1}{q^2-k^2}\right](z) \\ =& k^2\int_{-\infty}^{\infty}\mathrm{d}z\,\chi_V(z)\,e^{-ikz}\frac{ie^{ik|z|}}{2|k|} \\ =& \frac{ik}{2}\int_0^{\infty}\mathrm{d}z\,\chi_V(z)\left(e^{2ikz}+1\right), \end{aligned} \tag{S50}$$

where $\text{F.T.}^{-1}[]$ represents the inverse Fourier transform, and we have used the fact that $(q^2-k^2)^{-1}$ is the Fourier transform of the Green's function of the one-dimensional Helmholtz wave equation.

### C. Localization and Extended States

Here we discuss the predictions of our strong-contrast approximations that Anderson localization will generally be present in disordered non-stealthy layered media, whereas disordered stealthy hyperuniform layered media can be perfectly transparent within a finite range of wavenumbers. Perfect transparency implies an infinite localization length [18]. In both the non-scaled and scaled approximations [given in Eq. (S41) and Eq. (S44), respectively], the quantity $F^{(1\mathrm{D})}(k_q)$ is generally complex-valued at a given incident wavenumber $k_q$, producing a corresponding $\varepsilon_e^{\perp}(k_q)$ with a nonnegative imaginary part. Following conventional usage, a composite attenuates waves at a given wavenumber if the imaginary part of the effective dielectric constant is positive. Such attenuation occurs here only because of multiple scattering effects (not absorption). Employing a similar scaling analysis as in Ref. [4], if the spectral density of disordered layered media has the power-law scaling $\tilde{\chi}_V(k) \sim k^{\alpha}$ for small $k$, we can show that the imaginary part of the effective dielectric constant exhibits the following quasistatic behavior:

$$\begin{aligned} &\mathrm{Im}[\varepsilon_e^{\perp}(k_q)] \sim \mathrm{Im}[F^{(1\mathrm{D})}(k_q)] \\ \sim &\begin{cases} k_q, & \text{nonhyperuniform } (\alpha=0) \\ {k_q}^{1+\alpha}, & \text{non-stealthy hyperuniform } (\alpha>0) \end{cases}, \quad \text{as } k_q \to 0^+, \end{aligned} \tag{S51}$$

where nonhyperuniform systems take $\alpha = 0$, whereas non-stealthy hyperuniform ones take a positive but finite exponent, i.e., $0 < \alpha < \infty$. Thus, non-stealthy hyperuniform systems are less lossy than their nonhyperuniform counterpart. The scaling (S51) also yields the small-$k_q$ behaviors of the imaginary part of the effective wavenumber $k_e \equiv k_q\sqrt{\varepsilon_e^{\perp}(k_q)/\varepsilon_q}$:

$$\begin{aligned} &\mathrm{Im}[k_e] \sim k_q\,\mathrm{Im}[\varepsilon_e^{\perp}(k_q)] \\ \sim &\begin{cases} {k_q}^2, & \text{nonhyperuniform } (\alpha=0) \\ {k_q}^{2+\alpha}, & \text{non-stealthy hyperuniform } (\alpha>0). \end{cases} \end{aligned} \tag{S52}$$

We note that the scaling $\mathrm{Im}[k_e] \sim {k_q}^2$ for disordered nonhyperuniform systems is consistent with the prediction from the Lyapunov exponent [19]. Therefore, any disordered layered medium that

is not stealthy (i.e., $\tilde{\chi}_V(k) \neq 0$ for a finite range of $k$), whether hyperuniform or not, exhibits finite attenuation with $\text{Im}[\varepsilon_e^{\perp}] > 0$ for all positive wavenumbers. This implies that if such media are sufficiently large in size, all the incident waves are completely reflected back, i.e., Anderson localization can emerge.

By contrast, a similar analysis of both non-scaled and scaled approximations shows that 1D disordered stealthy hyperuniform packings defined by $\tilde{\chi}_V(k) = 0$ for $k < K$ have a finite range of wavenumbers of perfect transparency in the infinite-volume limit, i.e., $\text{Im}[\varepsilon_e^{\perp}] = 0$. The perfect transparency intervals predicted from the non-scaled and scaled approximations are given, respectively, by

$$0 \leq k_q < \frac{K}{2} = \rho\pi\chi, \tag{S53}$$

$$0 \leq k_q < K_T \equiv \frac{K}{2\sqrt{\langle\varepsilon\rangle}} = \frac{\rho\pi\chi}{\sqrt{\langle\varepsilon\rangle}}, \tag{S54}$$

where $\chi = K/(2\pi\rho)$ is the degree of stealthiness. We stress that these predictions are purely theoretical and hence do not rely on simulations or measurement of the spectral density. We show in Secs. 4 and 5 below that our theoretical predictions of the perfect transparency intervals, especially Eq. (S54), are in excellent agreement with the transmittance spectral ranges computed from FDTD simulations and the transfer matrix method; see Figs. S3 and S4. Importantly, the scaled formula (S44) also show excellent agreement with the ; see Fig. S6, We see that at the edges of the perfect transparency intervals, a discontinuous change occurs in $\text{Im}[\varepsilon_e^{\perp}]$ with $k_1$ (see Fig. S6), which was not observed in stealthy hyperuniform systems in higher dimensions [4]. Indeed, it is increasingly more difficult to achieve such a sharp change in $\text{Im}[\varepsilon_e^{\perp}]$ in higher dimensions because attenuation in $d$ dimensions results from scattering of all possible directions with a given incident wavenumber $k_1$ that involves an integral of $\tilde{\chi}_V(\mathbf{k})$ in a $(d-1)$-dimensional shell defined as $|\mathbf{k} - k_1\hat{\mathbf{z}}| = k_1$. In layered media, however, it is sufficient to consider the forward-scattering and backscattering contributions, i.e., $\tilde{\chi}_V(0)$ and $\tilde{\chi}_V(2k_1)$; see the imaginary part of $F^{(1D)}(k)$ given in Eq. (S45).

## 3. SIMULATIONS

### A. Collective-Coordinate Optimization Scheme

Here, we provide simulation parameters employed to generate 1D stealthy hyperuniform packings. In this work, instead of the standard collective-coordinate potential [20–22], we employ the revised one [4, 23, 24] that we described in the main text:

$$\Phi\left(\mathbf{r}^N\right) = \frac{1}{V_{\mathfrak{F}}} \sum_{|\mathbf{Q}|<K} S(\mathbf{Q}) + \sum_{i<j} u\left(r_{ij}\right), \tag{S55}$$

where $V_{\mathfrak{F}}$ is the volume of the fundamental cell $\mathfrak{F}$, and a soft-core repulsion term [25] is

$$u(r) = \begin{cases} (1 - r/\sigma)^2, & r < \sigma, \\ 0, & \text{otherwise.} \end{cases} \tag{S56}$$

We consider 1D stealthy hyperuniform packings of three $\chi$ values: $\chi = 0.1, 0.2$, and 0.3. For each $\chi$ value, we generate 5000 configurations of $N = 50$ particles and $\rho\sigma = 0.25$ from random initial point patterns. We then circumscribe each point with a hard rod of radius $a$ so that all systems have identical packing fraction $\phi_2 = 2\rho a = 0.2$. All of these packings are used to compute the spectral densities.

### B. FDTD Simulations

We confirm the accuracy of our predictions on transverse effective dynamic dielectric constant $\varepsilon_e^{\perp}(k_1)$ and *normal* transmittance of 3D disordered stealthy hyperuniform layered media by comparing them with the simulation results. For this purpose, we primarily rely on the finite-difference time-domain (FDTD) but use the transfer matrix method [26] to compute transmittance only in Fig. S3 because the transfer matrix method is not well suited for estimating the effective dynamic dielectric constant, which is central to our work, especially beyond the long-wavelength regime. For example, there are some techniques, including the Nicolson-Ross-Weir (NRW)

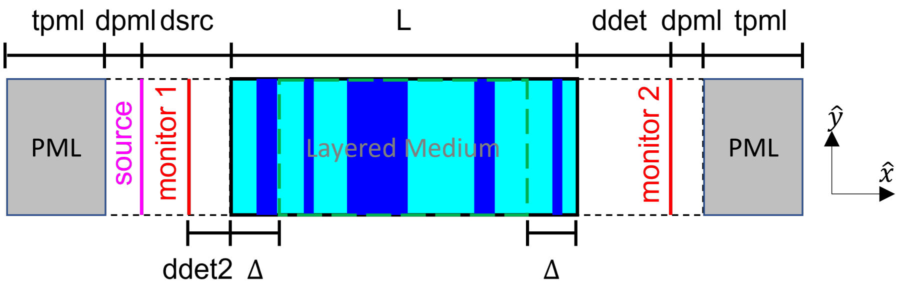


**Fig. S1.** Schematic of FDTD simulation setup for the two-phase layered media. For efficiency, simulations are performed in one dimension. A Gaussian pulse of the electric field generated from the source plane (shown in the magenta line) is incident into the media of length $L$ (inside a box with a black outline). We apply periodic boundary conditions along all directions but place the perfectly matched layers (PML, shown in the gray boxes) of thickness `tpml` at both ends of the simulation box to simulate the open boundary condition. Reflectance and transmittance spectra are measured on monitors 1 and 2 (shown in the red lines), respectively. In the homogenization procedure, we consider the fields in the region surrounded by a green dashed line.

**Table S1.** Length parameters of FDTD simulations depicted in Fig. S1. Length units are in $1/\rho$, where $\rho$ is the number density of 1D packings.

| Parameters | Values |
|---|---|
| tpml | $(0.05)^{-1}$ (longest wavelength) |
| dpml | 0.50 |
| dsrc | 3.00 |
| L | 50 |
| ddet | 3.00 |
| ddet2 | 1.50 |
| Δ | 0.50 |
| grid resolution | 100 pixels/$\rho$ |

procedure, that can be used to evaluate the electromagnetic properties of a homogeneous 'thin' film from scattering coefficients that the transfer matrix method can evaluate. However, these procedures do not apply well to dielectric composites without absorption that we study in this work for two reasons: (i) such estimations become more ambiguous for larger samples [27], which are required for the determination of well-defined effective properties. (ii) there are systematic errors due to the assumption of energy loss from attenuation, whereas there is no energy loss for our problem because attenuation is solely due to scattering.

Figure S1 shows the FDTD simulation setup. In this figure, the reference phase is shown in white, and its dielectric constant is identical to $\varepsilon_1 = 1$. For the particle phase, the dielectric constant is $\varepsilon_2 = 4$. The simulation parameters that we employed are listed in Table S1. Unlike the assumption in the Sec. 2, we set the wave to propagate along the $x$ axis to perform one-dimensional simulations.

We perform simulations for 400 distinct 1D stealthy hyperuniform packings of $N = 50$ and unit number density $\rho = 1$ at each $\chi$ value. The source plane generates a planar Gaussian pulse whose wavenumber spectrum spans from $0.05\rho$ to $4.05\rho$. We first perform a reference simulation without the layered media to record spectra of the incident flux, which is necessary to obtain the correct reflected intensity. We then run a regular simulation in the presence of a 1D configuration. Both reference and regular simulations last until the mean electric field at monitor 2 (Fig. S1) decays down to $10^{-7}$ of its maximum value. At the end of each regular simulation, we perform temporal

Fourier transformation to obtain electric field $E_y(x;\omega)$, dielectric displacement field $D_y(x;\omega)$, and reflected and transmitted intensities at a given set of frequencies $\omega$. The length scale $\Delta$ represents the regions that we excluded to minimize surface effects during the nonlocal homogenization method described in Sec. 3C.

### C. Nonlocal Homogenization Scheme

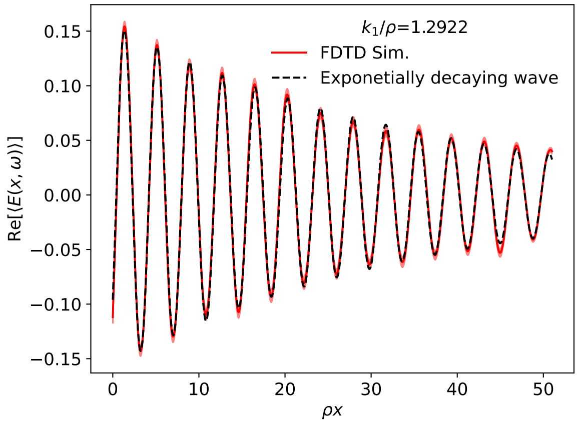


**Fig. S2.** Real part of an ensemble average of electric fields $\mathrm{Re}[\langle E_y(x,\omega)\rangle]$ inside 1D stealthy hyperuniform packings of $\chi = 0.2$, $\phi_2 = 0.2$, $N = 50$, and $\varepsilon_2/\varepsilon_1 = 4$. Here, the incident wavenumber is $k_1/\rho = 1.2922$, and 400 configurations are considered. Note that the effective medium description is accurate in that the electric field behaves like Eq. (S57) effectively.

Here, we describe the numerical homogenization method to extract the effective dynamic dielectric constant $\varepsilon_e^{\perp}(k_1)$ for the FDTD simulations, which is a minor revision of the method introduced in Ref. [4]. After performing the FDTD simulation for each packing as described in Sec. 3B, we obtain the electric field $E_y(x;\omega)$ and dielectric displacement field $D_y(x;\omega)$ for selected frequencies $\omega$. At each value of $\omega$ or, equivalently, $k_1(=\sqrt{\varepsilon_1}\omega/c)$, as shown in Fig. S2, we estimate the *effective wavenumber* $k_e$ from an ensemble average $\langle E_y(x;\omega)\rangle$ by curve-fitting an exponentially decaying sinusoidal function:

$$y = A\exp(-\,\mathrm{Im}[k_e]x)\cos\big(\mathrm{Re}[k_e]x + \eta\big). \tag{S57}$$

See Algorithm S1 for details. We then extract the effective dielectric constant $\varepsilon_e^{\perp}(k_1)$ from the nonlocal constitutive relation:

$$\varepsilon_e^{\perp}(k_1) = \langle \tilde{D}_y(k_e,\omega)\rangle \,/\, \langle \tilde{E}_y(k_e,\omega)\rangle\,, \tag{S58}$$

where $\langle \tilde{D}_y(k_e,\omega)\rangle$ and $\langle \tilde{E}_y(k_e,\omega)\rangle$ are the spatial Fourier transforms of $\langle D_y(x,\omega)\rangle$ and $\langle E_y(x,\omega)\rangle$ at $k_e$, respectively. We use 400 distinct packings to compute ensemble averages of fields. Estimated effective dielectric constants are compared to the theoretical predictions in Sec. 5.

**Algorithm S1.** Algorithm to find the effective wavenumber $k_e$ from ensemble averages of electric field $\langle E(x)\rangle$ and dielectric displacement field $\langle D(x)\rangle$ at a given frequency $\omega$ or, equivalently, $k_{\text{inc}} = \sqrt{\varepsilon_1}\omega/c$. We set $\epsilon = 10^{-2}$ and $x[0] = 0$. Here, $\lambda_e$ is the effective wavelength, and $\varepsilon_e(0) = \phi_1\varepsilon_1 + \phi_2\varepsilon_2$.

---

**Inputs:** 1D arrays of length $n$; $\{\langle E(x)\rangle, \langle D(x)\rangle, x$, and $\Delta x\}$ and float variables $\{\ k_{\text{inc}}$ and $\varepsilon_e(0)\ \}$
**Initialize:** $k_e \leftarrow 0.0 + 0.0i, \quad k_{\text{guess}} \leftarrow \sqrt{\varepsilon_e(0)}k_{\text{inc}}$
$E \leftarrow \text{Re}[\langle E(x)\rangle]$
$idx[] \leftarrow \{i \mid E[i] == 0\}$ ▷ Find zeros of the electric field
$len \leftarrow$ the length of $idx$
**if** $len < 3$ **then** ▷ Sample is shorter than $1.5\lambda_e$
    $\varepsilon_e \leftarrow$ Compute Eq. (S58) at $k_e = k_{\text{guess}}$
    $k_e \leftarrow \sqrt{\varepsilon_e}k_{\text{inc}}$
**else** ▷ Sample is longer than $1.5\lambda_e$
    $M \leftarrow n - 1$
    $E_{\text{normal}} \leftarrow \langle E(x)\rangle\ /\ \max|\langle E(x)\rangle|$
    **if** $\min_j |E_{\text{normal}}[j]| < \epsilon$ **then** ▷ If attenuation is strong,
        $M \leftarrow \min_l\{idx[l] \mid |E_{\text{normal}}[idx[l]]| < \epsilon\}$ ▷ field becomes too noisy beyond $x = x[M]$.
    **else** ▷ If attenuation is weak
        $M \leftarrow \max_j\{idx[j]\}$
    $k_i[0] \leftarrow \min_{j=idx[len-4],\ldots,M}\{-\ln\big(|E_{\text{normal}}[j]|\big)/x[j]\}$
    $k_i[1] \leftarrow \max_{j=idx[len-4],\ldots,M}\{-\ln\big(|E_{\text{normal}}[j]|\big)/x[j]\}$
    $\lambda_{\max} \leftarrow 2\max_{j=0,\ldots,M-1}\{x[idx[j+1]] - x[idx[j]]\}$
    $\lambda_{\min} \leftarrow 2\min_{j=0,\ldots,M-1}\{x[idx[j+1]] - x[idx[j]]\}$
    $k_r[0] \leftarrow 2\pi/\lambda_{\max}$
    $k_r[1] \leftarrow 2\pi/\lambda_{\min}$
    $x_{slice} \leftarrow x[idx[0],\ldots,M]$
    $E_{slice} \leftarrow E[idx[0],\ldots,M]$
    Fit Eq. (S57) to $x_{slice}$ and $E_{slice}$ with the constraints $k_r[0] \le \text{Re}[k_e] \le k_r[1]$ and $k_i[0] \le \text{Im}[k_e] \le k_i[1]$
    **return** $k_e$ ▷ Return the effective wavenumber

---

## 4. TRANSMITTANCE

**(a)**

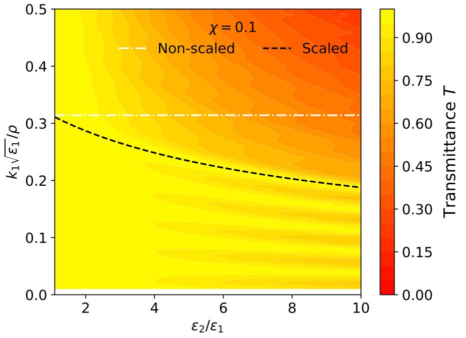


**(b)**

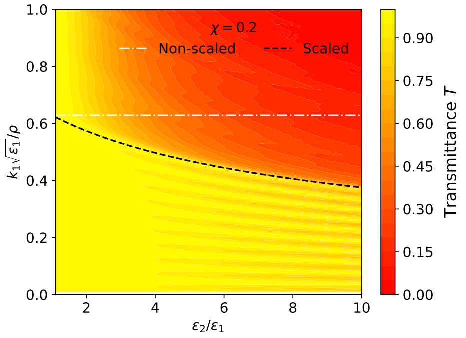


**(c)**

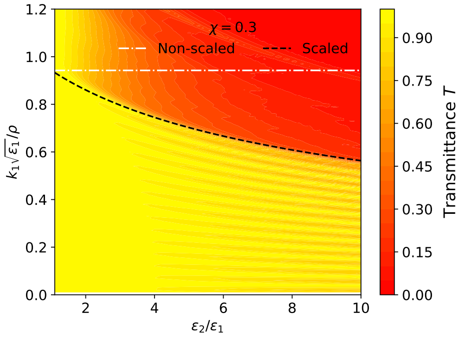


**Fig. S3.** Contour plots of the normal transmittance $T$ as a function of the phase contrast ratio $\varepsilon_2/\varepsilon_1$ and the dimensionless incident wavenumber $\sqrt{\varepsilon_1}k_1/\rho$ for disordered stealthy hyperuniform layered media of $\phi_2 = 0.2$ at three $\chi$ values: (a) $\chi = 0.1$, (b) $\chi = 0.2$, and (c) $\chi = 0.3$. We consider composites of $N = 50$ particles embedded in the reference phase of dielectric constant $\varepsilon_1$. Transmittance is evaluated via the transfer matrix method [26]. The white dot-dashed lines and the black dashed lines depict the upper bounds of the perfect transparency intervals by Eq. (S53) and Eq. (S54), respectively. The predictions from the scaled approximation show excellent agreement with the simulation results.

Here, we present some results of transmittance for stealthy hyperuniform media that are omitted in the main text. We begin by corroborating the predictions of the perfect transparency intervals given by Eq. (S53) and Eq. (S54) with the corresponding simulation results. We use the transfer matrix method [26] to compute the transmittance through disordered stealthy hyperuniform layered media of $\phi_2 = 0.2$ and $N = 50$ at $\chi = 0.1$, 0.2, and 0.3. At each $\chi$ value, we use 400 distinct configurations and span phase contrast ratio $\varepsilon_2/\varepsilon_1$ in the interval $[1.1, 10.0]$. Figure S3 shows the simulation results and two predictions of the perfect transparency intervals given by Eq. (S53) and Eq. (S54). The prediction from the scaled approximation (S54) very accurately captures the boundaries between high-transmittance (shown in yellow) and low-transmittance (shown in red) regions, whereas the non-scaled counterparts (S53) become increasingly inaccurate with $\varepsilon_2/\varepsilon_1$.

From both the non-scaled approximation (S41) and the scaled one (S44), we predict the *normal* transmittance $T$ through a layered medium at an incident wavenumber $k_1$ by assuming that the system is a homogeneous slab of thickness $L$ with an effective dielectric constant $\varepsilon_e^{\perp}(k_1)$ embedded in the reference phase of $\varepsilon_1$ and is optically thin so that waves inside it can interfere coherently. To estimate the normal transmittance, we use an Airy formula [26] of transmittance $T$ for a lossy

homogeneous slab with absorption:

$$T = \left| \frac{-\sqrt{\varepsilon_e^{\perp}}\, t^2 \exp\left(i\sqrt{\varepsilon_e^{\perp}} k_1 L\right)}{1 - r^2 \exp\left(2i\sqrt{\varepsilon_e^{\perp}} k_1 L\right)} \right|^2, \tag{S59}$$

where $r \equiv (1 - \sqrt{\varepsilon_e^{\perp}})/(1 + \sqrt{\varepsilon_e^{\perp}})$ and $t \equiv 2/(1 + \sqrt{\varepsilon_e^{\perp}})$, and is estimated using $\varepsilon_e^{\perp}$ from two formulas (S41) and (S44). Here, we also present an Airy formula for the reflectance $R$:

$$R = \left| r \left[ 1 - \frac{t^2 \exp\left(2i\sqrt{\varepsilon_e^{\perp}} k_1 L\right)}{1 - r^2 \exp\left(2i\sqrt{\varepsilon_e^{\perp}} k_1 L\right)} \right] \right|^2. \tag{S60}$$

In our nonlocal theory, the electric field inside the layered media attenuates solely due to multiple scattering but effectively behaves like a wave exponentially damped by absorption in a lossy homogeneous medium; see Fig. S2. Because the waves attenuated purely due to scattering are similar to those due to pure absorption, we expect the Airy formula (S59) to provide a good approximation, especially when scattering attenuation is weak. Even when the scattering attenuation is strong (e.g., outside of the perfect transparency intervals), the predictions using Eq. (S59) provide lower bounds on $T$ because the Airy formulas (S59) and (S60) always yield $T + R < 1$ for a lossy medium with $\text{Im}[\varepsilon_e^{\perp}] > 0$, whereas the simulation results give $T + R = 1$; see Fig. S4. However, such lower bounds on $T$ outside the perfect transparency intervals are still qualitatively accurate because $\varepsilon_e^{\perp}(k_1)$ of our formula is a physically feasible dielectric response due to the Kramers-Kronig relations (Sec. 6).

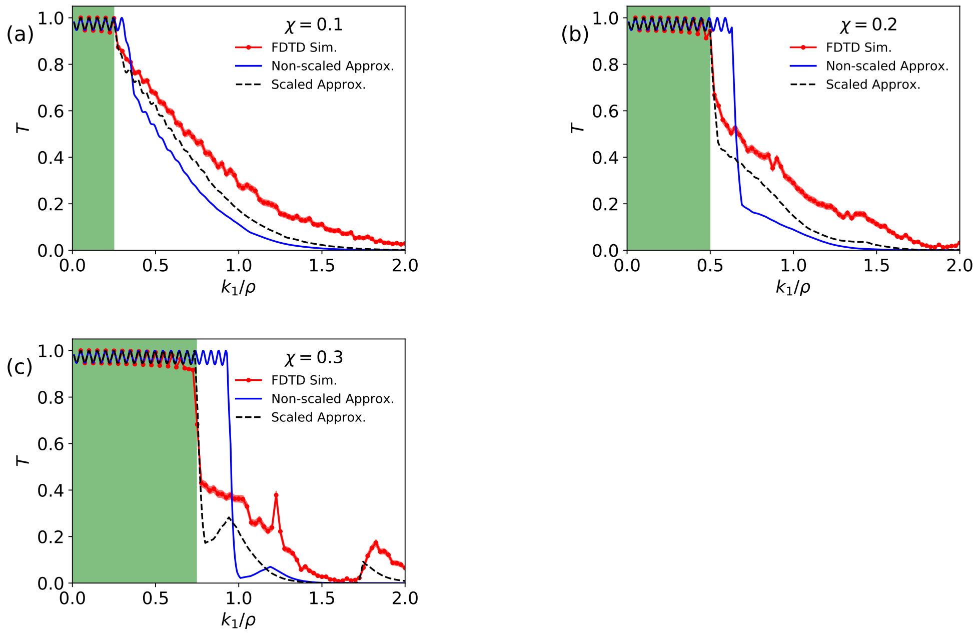


**Fig. S4.** Transmittance spectra $T$ as a function of the dimensionless wavenumber $k_1/\rho$ for disordered stealthy hyperuniform layered media of packing fraction $\phi_2 = 0.20$, particle number $N = 50$, and phase-contrast ratio $\varepsilon_2/\varepsilon_1 = 4$ at three values of (a) $\chi = 0.1$, (b) $\chi = 0.2$, and (c) $\chi = 0.3$. Composites are embedded in the reference phase of dielectric constant $\varepsilon_1$. The predictions of $T$ are computed by inserting the results of the non-scaled approximation (S41) and the scaled variant (S44) into Eq. (S59). The green-shaded areas illustrate the predicted perfect transparency intervals Eq. (S54). Because of no absorption, $T + R = 1$ in simulations, where $R$ is the reflectance.

We now compare our theoretical predictions for $T$ to corresponding results obtained from FDTD simulations for disordered stealthy hyperuniform layered media at $\chi = 0.1, 0.2$, and $0.3$; see

Fig. S4. This figure is identical to Fig. 5 in the main text but includes the predictions from the non-scaled approximation (S41). We clearly see that the scaled approximation (S44) very accurately predicts the perfect transparency intervals in which no Anderson localization is expected (green regions in Fig. S4), whereas the non-scaled approximation overestimates these intervals, as also shown in Fig. S3. For these reasons, we focus on the scaled approximation in the main text. Within these perfect transparency intervals ($k_1 < K_T$), the scaled approximation and simulation result coincide and show small-amplitude periodic oscillations in $T$ around unity [2], which come from coherent interference of the multiply reflected waves due to the finite system thickness $L$, and the periodicity is inversely proportional to $L$; see Fig. S5. However, such oscillations reduce to a constant close to unity when $L$ is much larger than the coherence length of light [26, 27]. Outside of the perfect transparency intervals, transmittance $T$ strongly depends on $L$: It is increasingly suppressed as $L$ increases and becomes virtually zero for sufficiently large $L$. Such a suppression results from the fact $\mathrm{Im}[\varepsilon_e^{\perp}(k_1)] > 0$ if $k_1 > K_T$, as shown in Fig. S5. Similarly, non-stealthy hyperuniform media are not perfectly transparent because $\mathrm{Im}[\varepsilon_e^{\perp}] > 0$ at any positive wavenumber $k_1$, as demonstrated in Sec. 7.

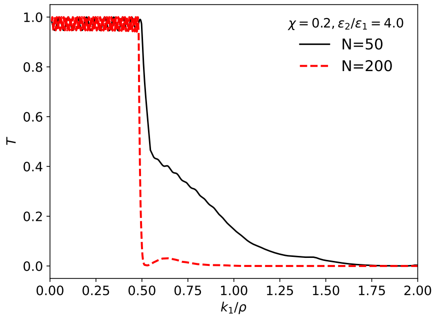


**Fig. S5.** Theoretical predictions of transmittance spectra $T$ as a function of the dimensionless wavenumber $k_1/\rho$ for disordered stealthy hyperuniform layered media of packing fraction $\phi_2 = 0.20$, phase-contrast ratio $\varepsilon_2/\varepsilon_1 = 4$, unit number density $\rho = 1$ and $\chi = 0.2$ at different system sizes $N = 50$ and 200. Composites are embedded in the reference phase of dielectric constant $\varepsilon_1$. The predictions of $T$ are computed from Eq. (S59) and the scaled approximation (S44). The perfect transparency interval is independent of $L = N/\rho$, and its edge becomes sharper as $L$ increases.

[2] These oscillations occur between $T = 4\langle\varepsilon\rangle/(1+\langle\varepsilon\rangle)^2$ and $T = 1$ [26].

## 5. EFFECTIVE DIELECTRIC CONSTANT

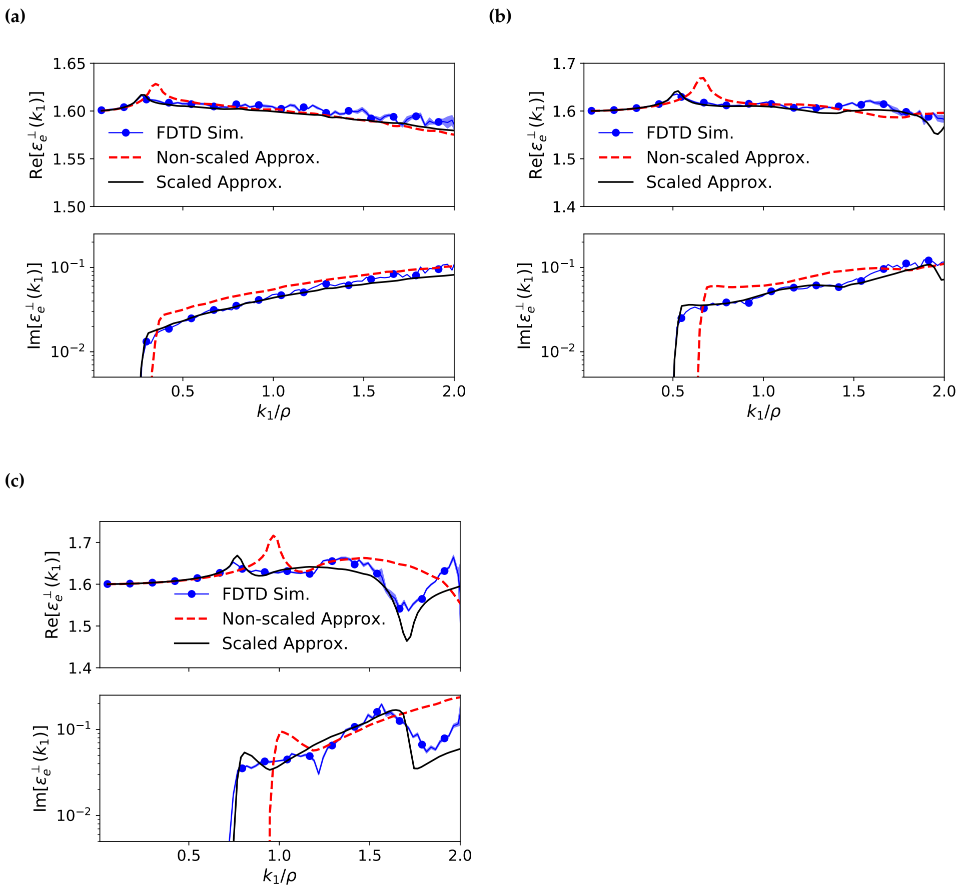


**Fig. S6.** Comparison of the predictions from the strong-contrast approximations for the effective dynamic dielectric constant $\varepsilon_e^\perp(k_1)$ of disordered stealthy hyperuniform (SHU) layered media as a function of the dimensionless wavenumber $k_1/\rho$ to the corresponding FDTD simulation results. We consider stealthy hyperuniform models of packing fraction $\phi_2(= 2\rho a) = 0.2$, particle number $N = 50$, unit number density $\rho = 1$, and phase-contrast ratio $\varepsilon_2/\varepsilon_1 = 4$ at three $\chi$ values: (a) $\chi = 0.1$, (b) $\chi = 0.2$, and (c) $\chi = 0.3$. Here, $k_1$ is the wavenumber in the reference phase. Theoretical predictions denoted by Non-scaled Approx. and Scaled Approx. are computed from Eq. (S41) and Eq. (S44), respectively. Note that Im[$\varepsilon_e$] on the lower panels are in a semi-log scale. Predictions show excellent agreement with the simulation results up to $k_1/\rho \lesssim 1.5$.

Here, we compare the effective dielectric constants from two strong-contrast approximations (S41) and (S44) to the results extracted from the FDTD simulations (see Sec. 3C). We consider 1D disordered stealthy hyperuniform packings of packing fraction $\phi_2 = 0.2$, particle number $N = 50$, and phase contrast ratio $\varepsilon_2/\varepsilon_1 = 4$ at three $\chi$ values: $\chi = 0.1, 0.2$, and 0.3. We extract the effective dielectric constant $\varepsilon_e^\perp$ from the FDTD simulations as described in Sec. 3C. Within the perfect transparency range, the values of Im[$\varepsilon_e^\perp$] extracted from the simulations are smaller than $5 \times 10^{-3}$ but have huge fluctuations. Considering the fact that Im[$\varepsilon_e^\perp$] $\neq 0$ within these intervals is inconsistent with the transmittance results shown in Fig. S4, one can see that such fluctuations are artifacts of finite-size effects: the system size $L = 50/\rho$ is too small to accurately determine Im[$k_e$] from curve fitting Eq. (S57) to weakly attenuated waves, which are virtually identical to sine waves. Both approximations well capture finite wavenumber ranges of perfect transparency in which Im[$\varepsilon_e$] $= 0$. While the non-scaled formula overestimates the sizes of these intervals, the scaled approximation very accurately predicts them, which is consistent with what we see from

the transmittance in Fig. S4. Furthermore, the scaled theory accurately predicts the positions of peaks in $\mathrm{Re}[\varepsilon_e^\perp]$ near the edges of the perfect transparency intervals. Predictions of $\varepsilon_e^\perp$ from the scaled approximation are very accurate up to $k_1/\rho \lesssim 1.5$. Because of such high predictive powers, we focus on the scaled approximation in the main text.

## 6. KRAMERS-KRONIG RELATIONS

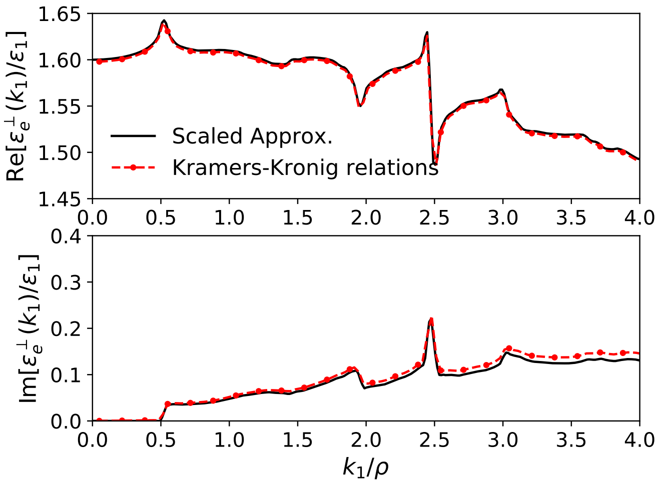


**Fig. S7.** Numerical verification of the Kramers-Kronig relations for the scaled strong-contrast approximation (S44). We consider 1D stealthy hyperuniform packing of $\chi = 0.2$, packing fraction $\phi_2 = 0.20$, and contrast ratio $\varepsilon_2/\varepsilon_1 = 4$. Here, $\rho$ is the number density. In the upper panel, we compare $\mathrm{Re}[\varepsilon_e(k_1)]$ of the approximation to that evaluated from the Kramers-Kronig relation Eq. (S61) and $\mathrm{Im}[\varepsilon_e(k_1)]$ of the approximation. In the lower panel, we compare $\mathrm{Im}[\varepsilon_e(k_1)]$ of the approximation to that evaluated from Eq. (S62) and $\mathrm{Re}[\varepsilon_e(k_1)]$ of the approximation. The predictions from the approximation and its transform via Kramers-Kronig relations show excellent agreement.

Here, we numerically show that our scaled strong-contrast approximation given in (S44) satisfies the Kramers-Kronig relations [28, 29], as does the corresponding approximation for 3D statistically isotropic media [4]:

$$\mathrm{Re}[\varepsilon_e(k_q)] = \varepsilon_q + \frac{2}{\pi}\mathrm{p.v.}\int_0^\infty \mathrm{d}q\, \frac{q\,\mathrm{Im}[\varepsilon_e(q)]}{q^2 - {k_q}^2}, \tag{S61}$$

$$\mathrm{Im}[\varepsilon_e(k_q)] = -\frac{2k_q}{\pi}\mathrm{p.v.}\int_0^\infty \mathrm{d}q\, \frac{\mathrm{Re}[\varepsilon_e(q)] - \varepsilon_q}{q^2 - {k_q}^2}, \tag{S62}$$

where p.v. stands for the Cauchy principal value of the integral. Both scaled and non-scaled strong-contrast approximations satisfy the Kramers-Kronig relations because the nonlocal attenuation function $F^{(1\mathrm{D})}(k)$ comes from $\boldsymbol{G}^{(q)}(\mathbf{x}-\mathbf{x}')$ given in Eq. (S7) that accounts for causality. The reader is referred to Ref. [4] for more theoretical discussion about the Kramers-Kronig relations for the strong-contrast approximations.

For illustrative purposes, we compare the effective dielectric constant $\varepsilon_e^\perp(k_q)$ from the scaled strong-contrast approximation (S44) to its transformation via the Kramers-Kronig relations. We consider 1D stealthy hyperuniform packing of $\chi = 0.2$, packing fraction $\phi_2 = 0.20$, and contrast ratio $\varepsilon_2/\varepsilon_1 = 4$; see Fig. S7. Specifically, in the upper panel of Fig. S7, we present the predictions of $\mathrm{Re}[\varepsilon_e(k_1)]$ from Eq. (S44) and those evaluated by using the Kramers-Kronig relation (S61) and $\mathrm{Im}[\varepsilon_e(k_1)]$ from the approximation. Similarly, in the lower panel, we compare $\mathrm{Im}[\varepsilon_e(k_1)]$ from the approximation with the calculation of Eq. (S62) by using $\mathrm{Re}[\varepsilon_e(k_1)]$ from the approximation. Computing the Kramers-Kronig relations, we carry out numerical integrals with an upper limit of $q = 74/\rho$. In both panels, the scaled strong-contrast approximation and its transformations via

the Kramers-Kronig relations show excellent agreement, which numerically confirms that our approximation satisfies these relations. Since the non-scaled approximation (S41) and the scaled one (S44) have identical functional form, the non-scaled formula also satisfies the Kramers-Kronig relations.

## 7. NON-STEALTHY HYPERUNIFORM LAYERED MEDIA

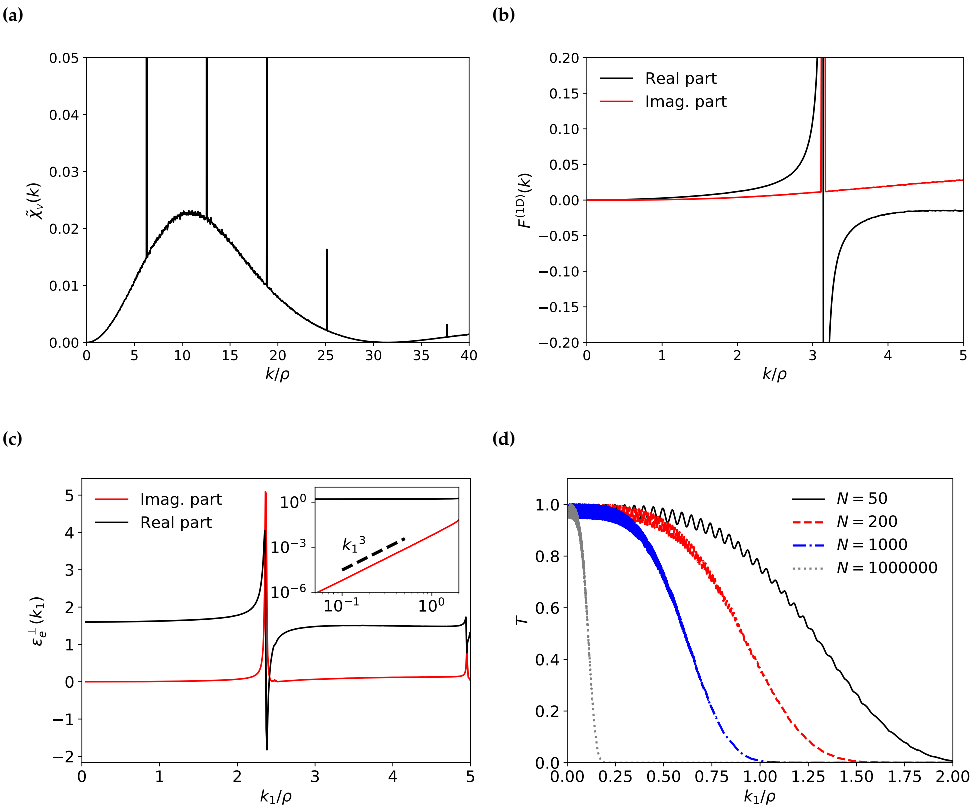


**Fig. S8.** Application of the scaled approximation (S44) to layered media derived from 1D URL of the maximum displacement $\Delta = 0.2/\rho$, packing fraction $\phi_2 = 0.2$, and phase contrast ratio $\varepsilon_2/\varepsilon_1 = 4$. (a) Spectral density $\tilde{\chi}_V(k)$ as a function of the dimensionless wavenumber $k/\rho$. (b) The real and imaginary parts of the nonlocal attenuation function $F^{(1D)}(k)$ as a function of $k/\rho$. (c) The effective dielectric constant as a function of the dimensionless incident wavenumber $k_1/\rho$ from the scaled approximation (S44). The inset is the log-log plot of the larger panel. (d) Transmittance $T$ using Eq. (S59) and the scaled approximation (S44) as a function of $k_1/\rho$ at various system sizes ($N = 50$, 200, 1000, and $10^6$).

Here, we demonstrate that non-stealthy hyperuniform layered media, characterized by $\tilde{\chi}_V(k) \neq 0$ for any finite range of wavenumbers, are not perfectly transparent by using our theoretical formula (S44). For this purpose, we consider 3D layered media derived from 1D *uniformly randomized lattice* (URL) model [30]. One can easily generate this model from the integer lattice by displacing each lattice point by a random vector that is uniformly distributed on the interval $[-\Delta, \Delta]$. Importantly, its structure factor $S(k)$ is known analytically [30–32]:

$$S(k) = 1 - \left[\frac{\sin(k\Delta)}{k\Delta}\right]^2 + \left[\frac{\sin(k\Delta)}{k\Delta}\right]^2 S_{\mathbb{Z}}(k)\,, \tag{S63}$$

where $S_{\mathbb{Z}}(k) \equiv (2\pi)\sum_{n=1}^{\infty}[\delta(k-2\pi n) + \delta(k+2\pi n)]$ is the structure factor of the integer lattice of unit spacing, implying that this model inherits Bragg peaks from the original lattice. Thus, we can investigate the effective wave properties of the URL models by using our formula (S44)

even without configurations. In this section, we set $\Delta = 0.2/\rho$ and create packings with packing fraction $\phi_2 = 0.2$ and dielectric constant $\varepsilon_2 = 4$ by circumscribing the points by identical rods of radius $a = 0.1/\rho$ without overlaps.

Figure S8 shows how we apply our scaled approximation (S44) to this 1D URL model step-by-step. We begin by computing the spectral density $\tilde{\chi}_V(k)$ from Eq. (S30) and Eq. (S63); see Fig. S8(a). This model is non-stealthy hyperuniform, and its spectral density has a power-law scaling $\tilde{\chi}_V(k) \sim k^2$ for small $k$. We then compute the nonlocal attenuation function $F^{(1D)}(k)$ from the spectral density and Eq. (S45); see Fig. S8(b). Inserting phase contrast ratio $\varepsilon_2/\varepsilon_1 = 4$, packing fraction $\phi_2 = 0.2$, and $F^{(1D)}(k)$ into Eq. (S44) yields the real and imaginary parts of the effective dielectric constant $\varepsilon_e^{\perp}(k_1)$; see Fig. S8(c). While we display this plot up to $k_1/\rho = 5$, this approximation is accurate up to $k_1/\rho \lesssim 1.5$. The inset in Fig. S8(c) shows a power-law scaling, $\mathrm{Im}[\varepsilon_e^{\perp}(k_1)] \sim {k_1}^3$ for small $k_1$ as predicted in Sec. 2 of the main text. Finally, we estimate the transmittance $T$ by using Eq. (S59) and the values of $\varepsilon_e^{\perp}(k_1)$ obtained in Fig. S8(c); see Fig. S8(d) at four system sizes $N = 50, 200, 10^3$, and $10^6$. We see that the 'effective' transparency interval, in which $T \approx 1$, shrinks with $N$ because $\mathrm{Im}[\varepsilon_e^{\perp}(k_1)]$ is small but nonzero at all wavenumbers. This figure clearly demonstrates that a perfect transparency interval that persists in the infinite-volume limit cannot exist for 1D non-stealthy hyperuniform media, despite these correlated disordered systems anomalously suppressing large-scale volume-fraction fluctuations.

## REFERENCES


1. S. Torquato, *Random Heterogeneous Materials: Microstructure and Macroscopic Properties* (Springer-Verlag, New York, 2002).
2. S. Torquato and G. Stell, "Microstructure of two-phase random media: I. The *n*-point probability functions," J. Chem. Phys. **77**, 2071–2077 (1982).
3. P. Debye, H. R. Anderson, and H. Brumberger, "Scattering by an inhomogeneous solid. II. The correlation function and its applications," J. Appl. Phys. **28**, 679–683 (1957).
4. S. Torquato and J. Kim, "Nonlocal Effective Electromagnetic Wave Characteristics of Composite Media: Beyond the Quasistatic Regime," Phys. Rev. X **11**, 021002 (2021).
5. M. C. Rechtsman and S. Torquato, "Effective dielectric tensor for electromagnetic wave propagation in random media," J. Appl. Phys. **103**, 084901 (2008).
6. A. Yaghjian, "Electric dyadic Green's functions in the source region," Proc. IEEE **68**, 248–263 (1980).
7. V. M. Agranovich and V. Ginzburg, *Crystal Optics with Spatial Dispersion, and Excitons* (Springer, Berlin, Heidelberg, 1984), 2nd ed.
8. A. V. Chebykin, A. A. Orlov, A. V. Vozianova, S. I. Maslovski, Y. S. Kivshar, and P. A. Belov, "Nonlocal effective medium model for multilayered metal-dielectric metamaterials," Phys. Rev. B **84**, 115438 (2011).
9. U. Frisch, "Wave propagation in random media," in *Probabilistic Methods in Applied Mathematics,* vol. 1 A. T. Bharucha-Reid, ed. (Academic Press, New York, 1968), pp. 75–198, 1st ed.
10. P. Sheng, *Introduction to Wave Scattering, Localization and Mesoscopic Phenomena* (Academic Press, New York, 1995).
11. L. Tsang, *Scattering of Electromagnetic Waves*, Wiley Series in Remote Sensing (Wiley, Chichester, UK, 2001).
12. A. Cazé and J. C. Schotland, "Diagrammatic and asymptotic approaches to the origins of radiative transport theory: Tutorial," J. Opt. Soc. Am. A **32**, 1475 (2015).
13. K. Vynck, R. Pierrat, R. Carminati, L. S. Froufe-Pérez, F. Scheffold, R. Sapienza, S. Vignolini, and J. J. Sáenz, "Light in correlated disordered media," arXiv:2106.13892 [cond-mat, physics:physics] (2021).
14. L. Tsang and J. A. Kong, "Scattering of electromagnetic waves from random media with strong permittivity fluctuations," Rádió Sci. **16**, 303–320 (1981).
15. T. G. Mackay, A. Lakhtakia, and W. S. Weiglhofer, "Strong-property-fluctuation theory for homogenization of bianisotropic composites: Formulation," Phys. Rev. E **62**, 6052–6064 (2000).
16. T. G. Mackay, A. Lakhtakia, and W. S. Weiglhofer, "Third-order implementation and convergence of the strong-property-fluctuation theory in electromagnetic homogenization," Phys. Rev. E **64**, 066616 (2001).
17. S. Torquato, "Hyperuniformity and its generalizations," Phys. Rev. E **94**, 022122 (2016).

18. F. M. Izrailev, A. A. Krokhin, and N. M. Makarov, “Anomalous localization in low-dimensional systems with correlated disorder,” Phys. Rep. **512**, 125–254 (2012).
19. A. M. Merzlikin and R. S. Puzko, “Homogenization of maxwell’s equations in a layered system beyond the static approximation,” Sci Rep **10**, 15783 (2020).
20. O. U. Uche, F. H. Stillinger, and S. Torquato, “Constraints on collective density variables: Two dimensions,” Phys. Rev. E **70**, 046122 (2004).
21. R. D. Batten, F. H. Stillinger, and S. Torquato, “Classical disordered ground states: Super-ideal gases, and stealth and equi-luminous materials,” J. Appl. Phys. **104**, 033504 (2008).
22. G. Zhang, F. Stillinger, and S. Torquato, “Ground states of stealthy hyperuniform potentials: I. Entropically favored configurations,” Phys. Rev. E **92**, 022119 (2015).
23. J. Kim and S. Torquato, “Multifunctional composites for elastic and electromagnetic wave propagation,” Proc. Nat. Acad. Sci. **117**, 8764–8774 (2020).
24. J. Kim and S. Torquato, “Effective elastic wave characteristics of composite media,” New J. Phys. **22**, 123050 (2020).
25. G. Zhang, F. H. Stillinger, and S. Torquato, “Can exotic disordered “stealthy” particle configurations tolerate arbitrarily large holes?” Soft Matter **13**, 6197–6207 (2017).
26. P. Yeh, *Optical Waves in Layered Media* (Wiley, Hoboken, NJ, 2005).
27. E. Nichelatti, “Complex refractive index of a slab from reflectance and transmittance: analytical solution,” J. Opt. A: Pure Appl. Opt. **4**, 400–403 (2002).
28. J. D. Jackson, *Classical Electrodynamics* (Wiley, New York, 1990).
29. G. W. Milton, D. J. Eyre, and J. V. Mantese, “Finite frequency range kramers-kronig relations: Bounds on the dispersion,” Phys. Rev. Lett. **79**, 3062–3065 (1997).
30. M. A. Klatt, J. Kim, and S. Torquato, “Cloaking the underlying long-range order of randomly perturbed lattices,” Phys. Rev. E **101**, 032118 (2020).
31. A. Gabrielli, “Point processes and stochastic displacement fields,” Phys. Rev. E **70**, 066131 (2004).
32. J. Kim and S. Torquato, “Effect of imperfections on the hyperuniformity of many-body systems,” Phys. Rev. B **97**, 054105 (2018).
